# Supplementary material for: The first-principles phase diagram of monolayer nanoconfined water
Source: arXiv:2110.14569 ancillary file (2022-07-05)
Supplement: Supplementary file 1 [file si.pdf]

# The first-principles phase diagram of monolayer nanoconfined water

Venkat Kapil,<sup>1,\*</sup> Christoph Schran,<sup>1,2,3</sup> Andrea Zen,<sup>3,4,5</sup> Ji  
Chen,<sup>6</sup> Chris J. Pickard,<sup>7,8</sup> and Angelos Michaelides<sup>1,2,3,†</sup>

<sup>1</sup>*Yusuf Hamied Department of Chemistry,  
University of Cambridge, Lensfield Road,  
Cambridge, CB2 1EW, United Kingdom*

<sup>2</sup>*Department of Physics and Astronomy,  
University College London, Gower Street,  
London, WC1E 6BT, United Kingdom*

<sup>3</sup>*Thomas Young Centre and London Centre for Nanotechnology,  
17-19 Gordon Street, London WC1H 0AH, United Kingdom*

<sup>4</sup>*Dipartimento di Fisica Ettore Pancini,  
Università di Napoli Federico II, Monte S. Angelo, I-80126 Napoli, Italy*

<sup>5</sup>*Department of Earth Sciences, University College London,  
Gower Street, London WC1E 6BT, United Kingdom*

<sup>6</sup>*School of Physics, Peking University, Beijing, 100871, China*

<sup>7</sup>*Department of Materials Science and Metallurgy,  
University of Cambridge, Cambridge CB30FS, United Kingdom*

<sup>8</sup>*Advanced Institute for Materials Research,  
Tohoku University, Sendai 980-8577, Japan*

---

\* Correspondence email address: vk380@cam.ac.uk

† Correspondence email address: am452@cam.ac.uk

## CONTENTS

|                                                   |    |
|---------------------------------------------------|----|
| S1. Methodology                                   | 4  |
| A. Selection of an accurate DFT functional        | 5  |
| B. Development of the machine learning potential  | 6  |
| 1. Committee Neural Networks in a nutshell        | 6  |
| 2. Automated development of the MLP               | 6  |
| 3. Validation of the MLP                          | 8  |
| C. Random Structure Search                        | 10 |
| D. Calculation of phase boundaries                | 13 |
| 1. Thermodynamic integration                      | 13 |
| 2. Coexistence simulations                        | 13 |
| E. Finite size effects                            | 15 |
| S2. Verification of key-findings                  | 16 |
| A. Verification of the MLP                        | 16 |
| B. The hexatic-like phase                         | 18 |
| C. The superionic phase                           | 19 |
| S3. Properties of water in the hexatic-like phase | 20 |
| A. Rotational relaxation time                     | 20 |
| B. Vibrational spectrum of hexatic water          | 21 |
| References                                        | 22 |

## S1. METHODOLOGY

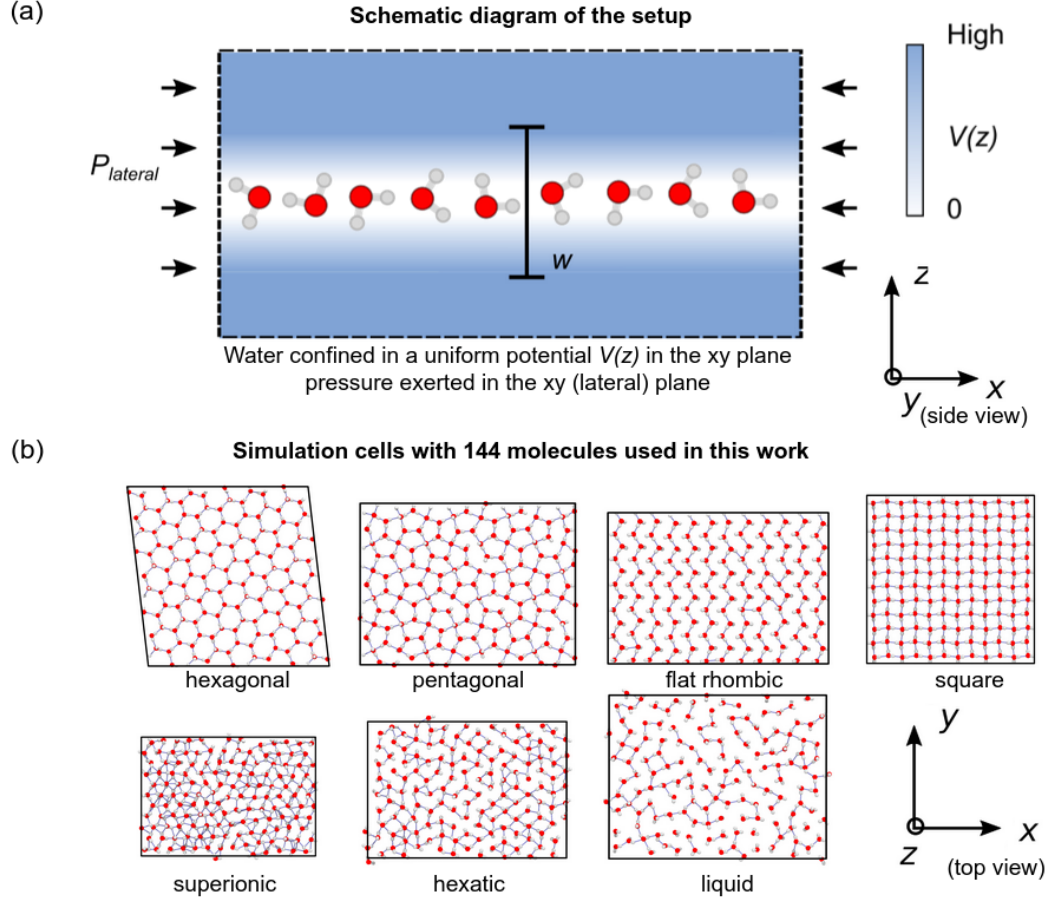

Figure S1. (a) A schematic diagram of the setup used to explore the phase behavior of monolayer nanoconfined water. (b) Simulation supercells containing 144 molecules periodic in the  $xy$  directions.

We split the total potential energy of the system, into graphene-water interactions modeled using a uniform 2D confining potential fitted to DMC water-graphene binding energies (taken from Ref. 1), and water-water interactions at DFT level. The confining potential only acts in the direction perpendicular to the plane of confinement, as in previous studies [2–5]. We model the lateral pressure – due to the vdW interactions pulling the graphene sheets and the termination of the edges – by applying an external lateral pressure within the  $NP_{xy}T$  ensemble. A schematic depiction of the setup and the physical interaction, and the actual simulation supercells are shown in Fig S1. The

methodology for calculation of the phase diagram is explained in the following subsections.

#### **A. Selection of an accurate DFT functional**

In order to select a DFT functional that accurately models the full range of interactions in monolayer confined water, we compare the relative enthalpies of a few known phases of monolayer water [1] – hexagonal, pentagonal, square and buckled-rhombic phases – with those calculated using fixed-node diffusion Monte Carlo (FN-DMC) in Ref. 3. FN-DMC has been shown to discern the stabilities of different bulk ice in excellent agreement with calorimetry results [6], and can thus be considered a reference for selecting appropriate DFT functionals.

We find that the revPBE0-D3 functional leads to the correct order of stabilities, and one of the smallest errors in relative enthalpies together with the HSE-vdW, and revPBE-vdW functionals [3]. Given that revPBE0-D3 is also known to describe the thermodynamic and dynamical properties of bulk water in excellent agreement with experimental results [7, 8], we select the revPBE0-D3 functional to further study the phase behavior of monolayer confined water.

The DFT reference calculations for the revPBE0-D3 functional were all performed with the CP2K simulation package [9] and its Quickstep module [10] using the same electronic structure setup for the revPBE0-D3 functional [11–14] employed in Ref. 15 for bulk water.

## B. Development of the machine learning potential

In order to explore the phase diagram of monolayer confined water, we have developed a machine learning potential trained to reproduce revPBE0+D3 reference calculations. For this development we make use of a recently introduced active learning protocol that is able to iteratively improve a MLP for previously unknown conditions as described in detail in Ref. 16.

### 1. *Committee Neural Networks in a nutshell*

Our MLP for water relies on Behler-Parrinello neural network potentials (NNPs) [17, 18] in order to form a committee neural network potential (C-NNP) [16] for active learning purposes. The NNP formalism has been successfully employed to understand the unique properties of water [8, 19], making it the ideal method for the current study. The main idea behind the C-NNP approach is the combination of multiple NNPs in a “committee model”, where the committee members are separately trained from independent random initial conditions to a subset of the total training set. While the committee average provides more accurate predictions than the individual NNPs, the committee disagreement, defined as the standard deviation between the committee members, grants access to an estimate of the error of the model. This committee disagreement provides an objective measure of the accuracy of the underlying model. To construct a training set of such a model in an automated and data-driven way, new configurations with the highest disagreement can be added to the training set. This is an active learning strategy called query by committee (QbC) and can be used to systematically improve a machine learning model. For further details on the C-NNP methodology we refer the reader to Ref. 16.

### 2. *Automated development of the MLP*

For the development of MLPs for various phase points we designed an active learning workflow, which is split into different generations. In each generation new state points are targeted to yield a NNP that will be used to generate new candidate structures for the next generation. This strategy

relies on the fact that a NNP model can faithfully yield configurations even for thermodynamic conditions not yet considered in the training set, if the conditions are not drastically different from those already considered. Within a generation, QbC is used to adaptively extend the training set by selecting the most representative configurations separately for each state point, improving its description. With this procedure, multiple state points can easily be treated in parallel. At the very beginning of each QbC cycle, a small number of random configurations is chosen to train the first committee, while in subsequent iterations, new configurations are selected based on the highest atomic force committee disagreement. Convergence of these individual QbC cycles can be detected by monitoring this disagreement. Once all QbC cycles for the selected conditions in a given generation are converged, the individual training sets are combined and a final tight optimization of that generation’s resulting NNP is performed.

Using this workflow, a condensed phase water model at revPBE0-D3 level has been developed in Ref. 16 for liquid water at ambient and elevated temperatures and pressures as well as for different phases of ice, and the air-water interface — all including nuclear quantum effects. In this work, we used this model as the starting point and added new configurations to the training set, which have been identified in two additional generations. In the first generation, 15 distinct conditions were targeted by individual active learning cycles. These consist of NpT simulations at 100, 250, and 400 K of monolayer and bilayer water, bulk water and hexagonal ice, ice VII and VIII at high pressures, and finally PIMD NpT simulations of monolayer water at 400 K. For each temperature, pressures of 0.1, 12.7, 143.8 to 885.9 MPa were combined in one active learning cycle, except for ice VII and VIII for which 885.9, 1623.8, 2976.4, 5455.6, 10000.0 MPa were selected. In addition, two sets of structures obtained during AIRSS for mono- and bilayer ice [1, 20] were also used in separate active learning cycles. Overall, 521 new structures from these various conditions were added to the training set of the model. In the next generation we performed NpT pressure ramp simulations, again at 100, 250, and 400 K, for monolayer water up to pressures of 5-7 GPa, depending on the temperature. In addition to a classical description of the nuclei, we also performed the same simulations with quantum nuclei, resulting in 6 distinct conditions which have been targeted by separate active learning cycles. During these cycles 207 additional structures were identified and added to the training set.

### 3. Validation of the MLP

The final training set of our model consists of 1542 structures used to train the NNP model for the exploration of the phase diagram of monolayer confined water. For this final model we have used only a single NNP for performance considerations and have switched to a larger set of symmetry functions that has been optimized for the description of water. [21] This switch has led to a more stable performance of the model beyond pressures of 7 GPa and has also slightly improved the force and energy accuracy of the model, which we attribute mainly to the better resolution of this set of symmetry functions.

We obtain an energy and force root mean square error (RMSE) for the training set of 2.4 meV per H<sub>2</sub>O (or 0.2 kJ/mol) and 75.4 meV/Å, respectively. These errors are consistent with the MLP predictions of 0 K static lattice energies of the known phases at 0 pressure and 2 GPa, as tabulated in table S1, which on average are within 0.2 kJ/mol of the DFT reference. To test the performance of the model across the a wide range of temperature and pressure, we build an out-of-sample test set by drawing configurations from simulations of a disordered phase at 20 - 600 K and 0 - 4 GPa. The largest force RMSE for this test set is with 100 meV/Å, suggesting that the model remains accurate and robust across a wide range of temperature and pressure.

In order to validate that the model keeps its excellent performance for the original condensed phase conditions, we have determined the equilibrium density of water at 300 K and 1 bar from NpT simulations. We obtain a density of 0.93 kg/L which is in very good agreement with the densities obtained for the same functional [8, 22]. In addition, we have determined the melting temperature of ice Ih to liquid water with our model. For this purpose, we have used interface pinning to get the solid-liquid free energy using the qtip4p/f force field model [23], and further used thermodynamic integration to promote this from the force field baseline to the NNP level. We have also included corrections arising from quantum nuclear and finite size effects, based on previous work

that use MLPs trained on revPBE0-D3 [8, 24]. From this we estimate a melting point of  $270 \pm 5$  K, in good agreement with the experimental result, and with other MLPs based on revPBE0-D3 [8].

| Polymorph    | Lattice Enthalpy |     |     |          |     |     |
|--------------|------------------|-----|-----|----------|-----|-----|
|              | [kJ/mol]         |     |     |          |     |     |
|              | At 0 GPa         |     |     | At 2 GPa |     |     |
|              | DFT              | NNP | DMC | DFT      | NNP | DMC |
| Hexagonal    | 0                | 0   | 0   | -        | -   | -   |
| Pentagonal   | 0.5              | 0.2 | 0.4 | 4.8      | 4.5 | 3.3 |
| Flat-Rhombic | 2.3              | 1.3 | 2.2 | 0        | 0   | 0   |
| Square       | 3.0              | 3.1 | 1.5 | 3.0      | 1.8 | 1.0 |

Table S1. Relative lattice enthalpies of different polymorphs of monolayer confined water calculated using revPBE0-D3 (DFT), the corresponding MLP developed in this work, and FN-DMC (DMC) – the reference level of theory used to select the DFT functional. FN-DMC values have been taken from Ref. 3 for all structures, except for the newly found flat-rhombic phase which was computed as part of this study using exactly the same computational settings as in Ref. 3. The dashed entries (-) suggest that the structure is not stable at the indicated pressure.

### C. Random Structure Search

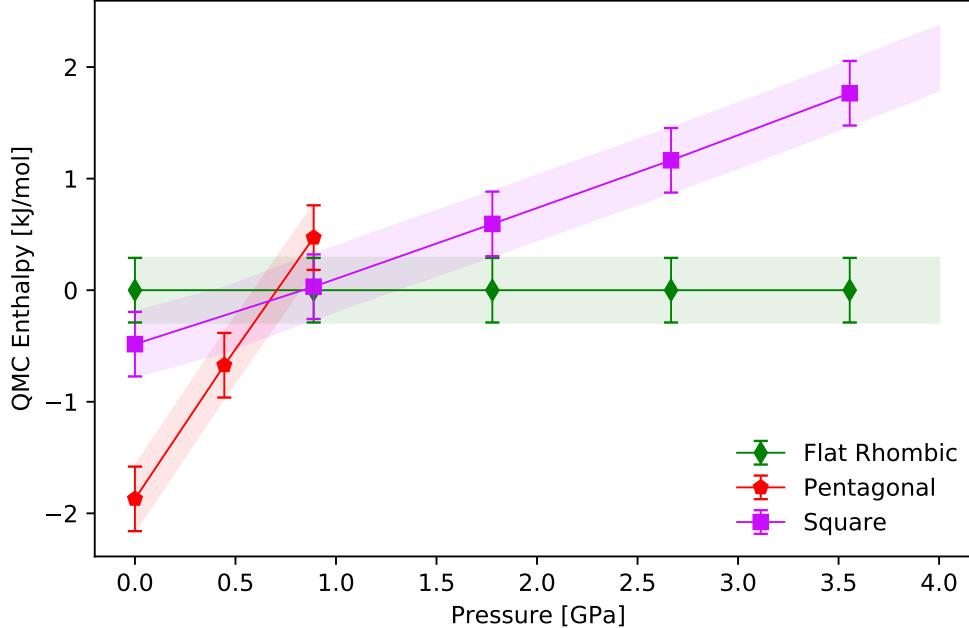

Figure S2. The pressure dependence of the lattice enthalpies of the pentagonal (red) and square (pink) phases relative to the flat-rhombic (green) phase using FN-DMC. Error bars indicate stochastic DMC error.

Within our random structure search (RSS), polymorphs of monolayer ice are probed by randomly placing water molecules within the confinement regions, subject to boundary conditions that prevent atoms from overlapping. The unit cell (in the xy direction) and the positions of these "random" configurations are optimized using the MLP and the confinement potential at different lateral pressures. This procedure is repeated for different unit cell sizes with 2, 4, 6, 8, 10, 12, 18, 24, 36 and 72 water molecules with confinement widths from 5-8 Å for pressures from 0 to 4 GPa. We are able to recover all previously known monolayer ice polymorphs – the hexagonal, pentagonal, buckled-rhombic and square phases. In addition, we found a new flat-rhombic phase in high-pressure searches to be more stable than the square phase.

The relative stabilities of all (relevant) polymorphs at FN-DMC level are summarized in Table S1.

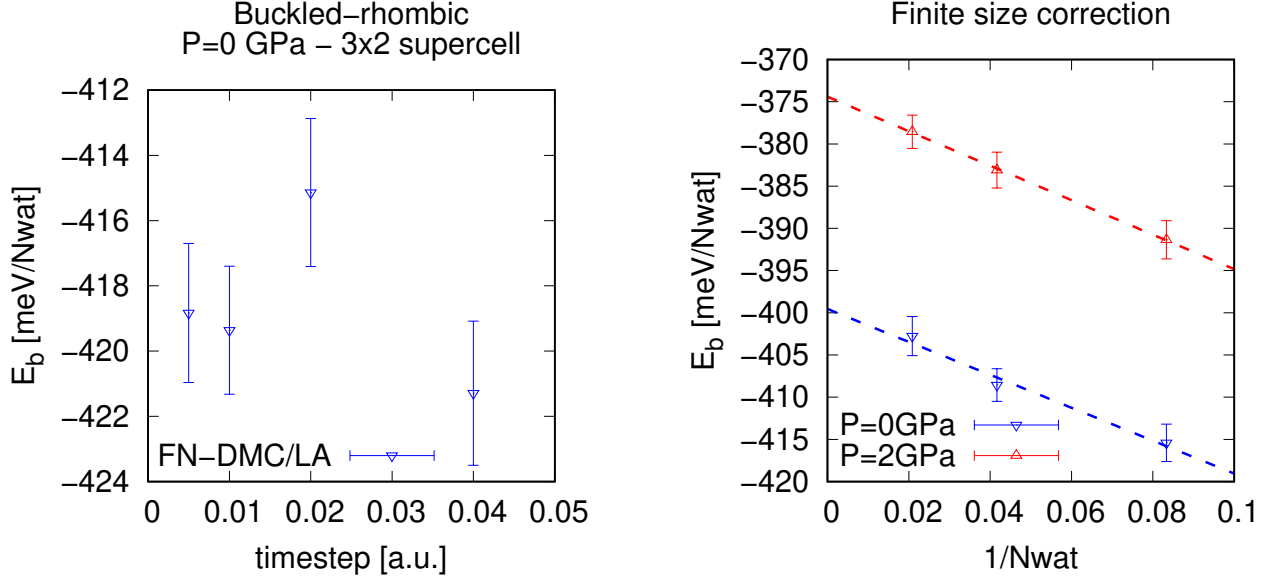

Figure S3. Left: Timestep dependence in the DMC binding energy  $E_b$  for the new buckled-rhombic polymorph (at zero pressure and on a  $3 \times 2$  supercell), using the setup discussed in the text. Right: Extrapolation of the binding energy  $E_b$  for infinite system, as obtained assuming the finite size error is proportional to the inverse of the number of water molecules  $N_{\text{wat}}$  in the simulated supercell. This approach is the same used in Ref. [3]

Pressure dependence of the relative stabilities, as shown in Fig. S2, reveals the competing nature of the square and rhombic phases. We find that between 0.8 and 2.0 GPa square and rhombic phases are near degenerate (to within the statistical errors of DMC), while beyond 2 GPa at 0 K the flat-rhombic phase is the most stable one.

DMC simulations have been performed using the CASINO package [25, 26], using Dirac-Fock pseudopotentials [27, 28] with the locality approximation [29]. Slater-Jastrow trial wave functions with single Slater determinants were used and the single particle orbitals obtained from DFT-LDA plane wave calculations reexpanded in terms of B-splines [30]. We used the DMC algorithm with the prescriptions of Ref. [31], which allows a DMC time step as large as 0.02 a.u. to be used with negligible time step errors, as observed in Ref. [3] and tested here on the new flat-rhombic polymorph, see

figure S3. The finite size errors on the DMC energies for the periodic systems have been corrected by extrapolating to the infinite system limit based on the evaluations at growing supercell size, as explained in Ref. [3]. The lattice energy for the new flat-rhombic polymorph was estimated separately for the configurations at zero pressure and at 2 GPa, in each case, the  $3 \times 2$ ,  $4 \times 3$  and  $6 \times 4$  supercells, see figure S3.

## D. Calculation of phase boundaries

The solid-solid phase boundaries were calculated using the thermodynamic integration technique [32, 33], and the solid-disordered phase-boundaries were calculated from coexistence simulations [34] as detailed in the following subsections.

### 1. Thermodynamic integration

At each pressure, we begin by calculating the classical harmonic Helmholtz free energy at 20 K ( $A_{20K}^{\text{harm}}$ ) of a given polymorph, and perform a harmonic-to-anharmonic thermodynamic integration to estimate the classical anharmonic Gibbs free energy [33]

$$G(P, T_{20K}) = A_{20K}^{\text{harm}} + \Delta A_{20K}^{\text{anharm}} + PV + k_B(20K) \ln p(V)_{P,20K}, \quad (1)$$

where,  $V$  is the volume of the structure optimized at pressure  $P$ , and  $p(V)_{P,20K}$  is the probability of observing volume  $V$  at 20 K and pressure  $P$ . The temperature dependent Gibbs free energy is estimated from a thermodynamic integration over temperature

$$\frac{\partial G(P, T)/T}{\partial T} = -\frac{H(P, T)}{T^2}, \quad (2)$$

up to the temperature at which the phase becomes disordered. The phase diagram for the polymorphs is calculated by identifying the phase with the lowest Gibbs free energy at each  $P, T$ .

### 2. Coexistence simulations

To estimate solid-disordered phase boundaries we perform co-existence simulations at different pressures, over a range of temperatures (intervals of 10 K) estimated from the simulations at which polymorphs become disordered. The initial configurations for the coexistence simulations are performed carefully in 3 steps:

1. We create a 2x1x1 simulation cell and thermalize at  $P, T$ ,

2. We fix the oxygen atoms in one-half the cell, and perform a high temperature simulation to melt the other-half of the cell in the NVT ensemble (with constraints), and a short simulation to cool the disordered phase to  $T$  in the NVT ensemble (with constraints),
3. We perform a short equilibration within the  $NP_xT$  simulation to relax the densities of the solid and liquid phases.

We then perform a 2 ns long production within the  $NP_xT$  simulation and monitor the migration of phase boundaries. At each pressure, the lowest temperature at which we do not observe any melting is considered the melting temperature, and it is assigned an uncertainty of 10 K.

### E. Finite size effects

To understand how finite size effects influence phase boundaries, we perform nanosecond long temperature sweeps at across the pressure range for different system sizes. Specifically, we study the melting of monolayer hexagonal phase at 0 pressure, pentagonal phase at 0.5 GPa and flat-rhombic phase at 1 GPa. As shown in Fig. S4, increasing the number of water molecules from 32 to 288 for hexagonal ice, and from 48 to 432 for pentagonal ice merely shifts the temperature at which the structures melts merely by 20 K. In the case of flat-rhombic ice, the temperature at which the structure melts into a hexatic-like phase, only changes by 20 K on increasing the number of molecules from 144 to 384. Overall, these results suggest that our simulation cells – containing 144 molecules of water for all phases – exhibit a small finite size effects that are of the order of the errors of the coexistence simulations.

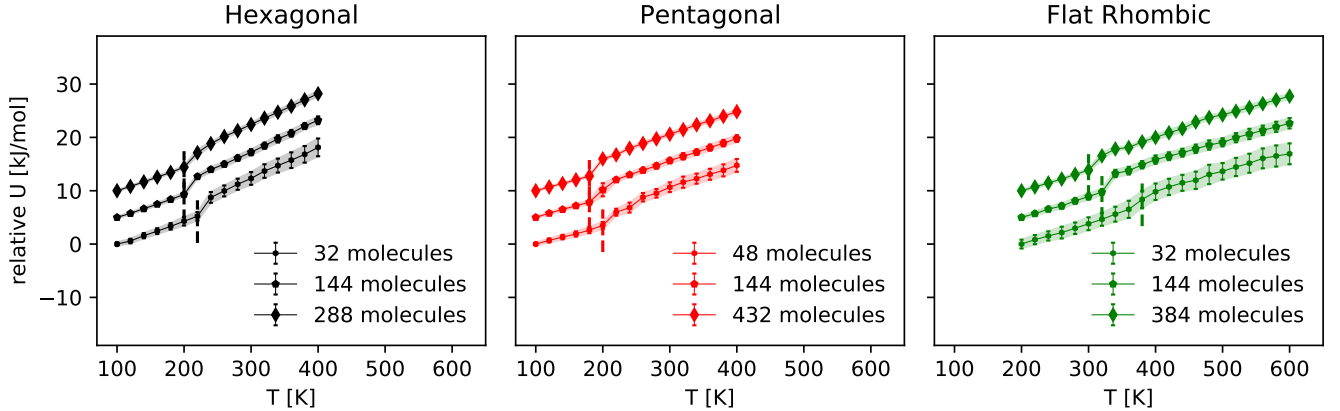

Figure S4. The temperature dependence of the potential energy for simulations initialized with monolayer hexagonal, pentagonal and flat-rhombic ice phases simulations at 0 pressure, 0.5 GPa and 1.0 GPa respectively. The number of water molecules in the simulation cell are indicated in the legend, with larger (smaller) marker sizes corresponding to larger (smaller) system sizes. The potential energy of the curves have been translated vertically to make it easier to discern the temperature of melting (indicated by a vertical dashed line) for different systems sizes. Shaded regions indicate statistical uncertainty.

## S2. VERIFICATION OF KEY-FINDINGS

### A. Verification of the MLP

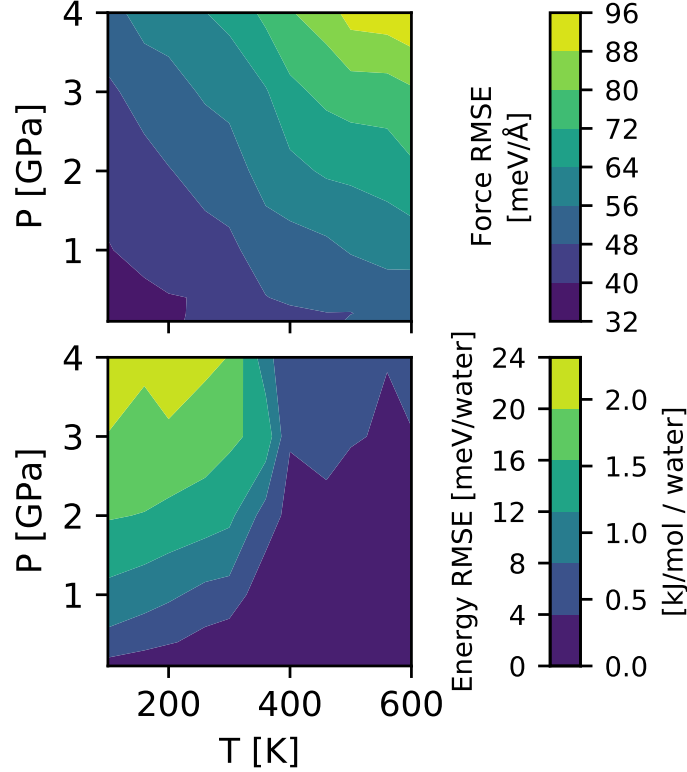

Figure S5. Force (top) and energy (bottom) root mean square error (RMSE) of an independent validation set covering the explored phase diagram of mono-layer confined water.

To rule out the possibility that the hexatic-like and superionic phases are not because of problems with the MLP, we study the energy and force RMSEs for the new (and thus out-of-sample) flat-rhombic phase across the full phase diagram. We sample configurations from simulations at  $P, T$  grid points of the phase diagram with pressures of 0.1, 100, 200, 400, 1000, 2000, 3000, and 4000 MPa and temperatures of 100, 160, 200, 260, 300, 360, 400, 460, 500, 560, and 600 K. At every grid point 10 random structures were extracted in order to compute the revPBE0-D3 reference energy and forces for these configurations. The resulting comprehensive validation set allows us to provide a full overview of the performance of our NNP model over the entire phase diagram. This performance

assessment is presented in Fig. S5. Overall, our model provides convincing accuracy across the entire phase diagram with only slightly larger force RMSE values at high temperatures and pressures. The largest observed values on the order of 100 meV are still similar to or lower than those reported for other water models. [8]. This highlights the good performance of our model and thus the validity of the reported findings in the main text.

## B. The hexatic-like phase

AIMD test simulations were also carried out with the CP2K package using both the revPBE0-D3 and the revPBE-D3 functionals. A Nosé-Hoover chain thermostat was used to simulate an NVT ensemble. A timestep of 1 fs was used and the mass of hydrogen was set as deuterium. The model consists of two layers of graphene and an embedded layer of 2D ice. The superionic and the hexatic-like structures were stretched slightly ( $< 10\%$ ) to fit the lattice of graphene supercells. In each graphene layer, 8 evenly distributed atoms were not allowed to move along the perpendicular direction during the AIMD simulations to avoid buckling. The DZVP-MOLOPT-SR basis set was used for C and the TZV2P basis set was used for O and H. Auxiliary density matrix method was employed in the revPBE0-D3 simulations. An energy cutoff of 400 Ry was used in all simulations.

A layer of the hexatic-like phase consisting of 16 water molecules is confined in two layers of graphene separated by 5 Å. The supercell, including the vacuum slab, is  $12.3 \times 8.52144 \times 20.0$  Å in three dimensions. We perform simulations for the hexatic-like structure at 400 K for 20 ps and 10 ps using the revPBE-D3 and the revPBE0-D3 functional, respectively. During all the simulations, we do not observe protonization of graphene, and all atoms in water molecules remain in the hexatic-like 2D water layer (Fig. S6 ). Moreover we observe rotation of the water molecules in agreement with the predictions of the MLP together with the confinement potential.

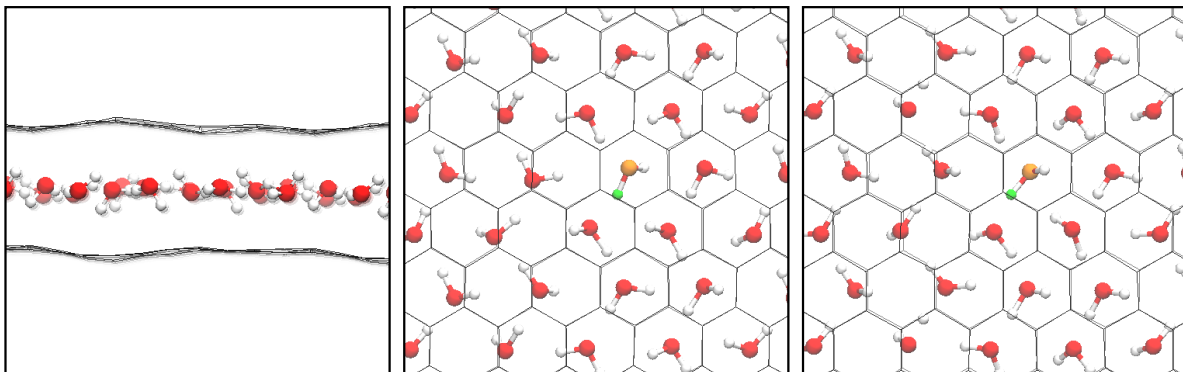

Figure S6. A snapshot from the revPBE-D3 AIMD simulation of the hexatic-like phase confined in explicit graphene. Left: the side view; middle: the top view at 10 ps; right: the top view at 20 ps. The orange and green spheres highlight one oxygen and one proton, which are bonded

### C. The superionic phase

Test AIMD simulations are also carried out for the superionic phase confined in explicit graphene layers. The supercell is  $9.84 \times 8.52144 \times 20.0$  Å in three dimensions and consists of 16 water molecules. We perform simulations for the superionic phase at 600 K. The trajectories are collected for 50 ps and 10 ps with the revPBE-D3 functional and the revPBE0-D3 functional, respectively. During all the simulations, we observe a significant amount of proton transport events, but all atoms remain in the water layer and do not attach to graphene (Fig. S7).

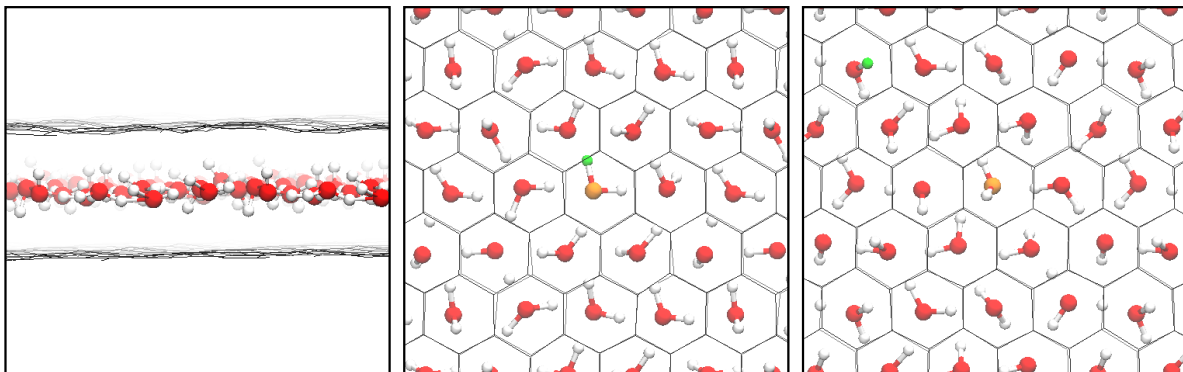

Figure S7. A snapshot from the revPBE-D3 AIMD simulation of the superionic phase confined in explicit graphene. Left: the side view; middle: the top view at 10 ps; right: the top view at 50 ps. The orange and green spheres highlight one oxygen and one proton, which are bonded at 10 ps and are separated at 50 ps.

### S3. PROPERTIES OF WATER IN THE HEXATIC-LIKE PHASE

#### A. Rotational relaxation time

The rotational relaxation (reorientation) dynamics can be calculated on the basis of the orientation time correlation functions. Here we estimate the 1st order orientational autocorrelation function for the O–H molecular axis of the hexatic-like phase at 1 GPa from 340 to 400 K using

$$C_1(t) = \langle P_1[v(0) \cdot v(t)] \rangle, \quad (3)$$

where,  $v(t)$  is the orientation of the O–H bond at time  $t$ , and  $P_1$  is the Legendre polynomial of degree one. The corresponding rotational relaxation time is given by the integral of the orientational autocorrelation function. As shown in Fig. S8,  $C_1(t)$  decay rapidly to 0 for the hexatic-like phase (beyond 320 K). The relaxation time at 340 K is around seven times smaller than that of room temperature liquid water, indicating facile rotation of water molecules in the hexatic-like phase.

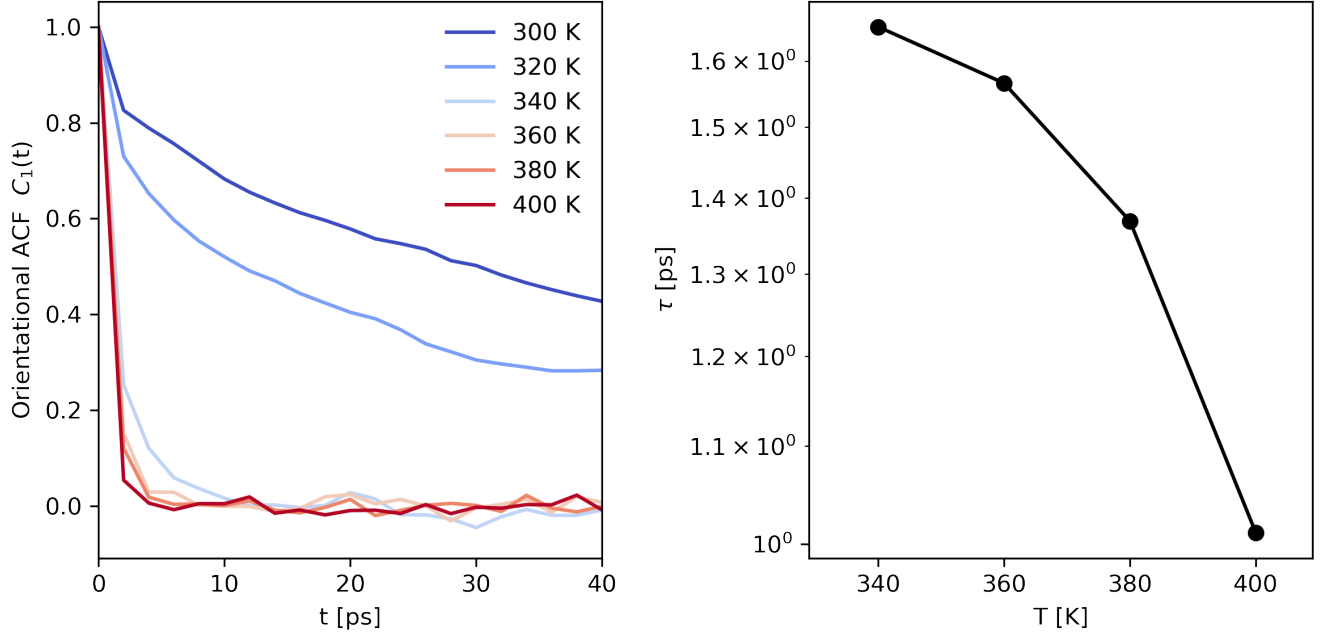

Figure S8. Left: 1st order orientational autocorrelation function of the hexatic phase at 1 GPa from 340 to 400 K. Right: Temperature dependence of the 1st order orientational relaxation time for the O–H molecular axis of the hexatic phase at 1 GPa.

## B. Vibrational spectrum of hexatic water

We estimate the vibrational spectra across the flat-rhombic to the hexatic-like phase transition from the power spectrum of the velocity autocorrelation function. As shown in Fig. S9, the flat-rhombic phase of monolayer water is characterized by two distinct vibrational bands for hydrogen bonded and dangling O–H bonds, and clear features for the librational modes. On the other hand, the rotations in the hexatic-like phase merge the two stretching bands into a doublet, and smear out the fine structure of the librational band.

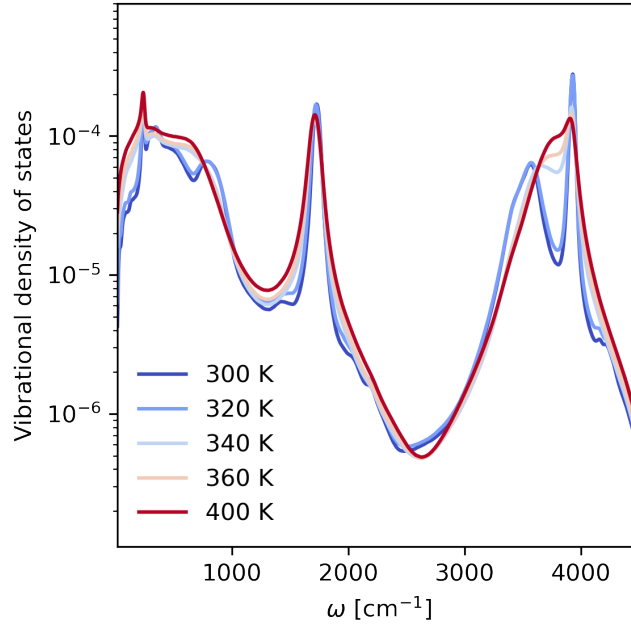

Figure S9. The vibrational spectra across the flat-rhombic (up to 320 K) to the hexatic-like phase transition (beyond 340 K) as calculated by the Fourier transform of the velocity autocorrelation function.

## REFERENCES

- [1] J. Chen, G. Schusteritsch, C. J. Pickard, C. G. Salzmann, and A. Michaelides, *Physical Review Letters* **116**, 025501 (2016).
- [2] F. Corsetti, P. Matthews, and E. Artacho, *Scientific Reports* **6**, 18651 (2016).
- [3] J. Chen, A. Zen, J. G. Brandenburg, D. Alfè, and A. Michaelides, *Physical Review B* **94**, 220102 (2016).
- [4] S. Li and B. Schmidt, *Physical Chemistry Chemical Physics* **21**, 17640 (2019).
- [5] Y. Zhu, F. Wang, and H. Wu, *The Journal of Chemical Physics* **146**, 134703 (2017).
- [6] A. Zen, J. G. Brandenburg, J. Klimeš, A. Tkatchenko, D. Alfè, and A. Michaelides, *Proceedings of the National Academy of Sciences* **115**, 1724 (2018).
- [7] O. Marsalek and T. E. Markland, *The Journal of Physical Chemistry Letters* **8**, 1545 (2017).
- [8] B. Cheng, E. A. Engel, J. Behler, C. Dellago, and M. Ceriotti, *Proceedings of the National Academy of Sciences* **116**, 1110 (2019).

- [9] T. D. Kühne, M. Iannuzzi, M. Del Ben, V. V. Rybkin, P. Seewald, F. Stein, T. Laino, R. Z. Khaliullin, O. Schütt, F. Schiffmann, D. Golze, J. Wilhelm, S. Chulkov, M. H. Bani-Hashemian, V. Weber, U. Borštnik, M. Taillefumier, A. S. Jakobovits, A. Lazzaro, H. Pabst, T. Müller, R. Schade, M. Guidon, S. Andermatt, N. Holmberg, G. K. Schenter, A. Hehn, A. Bussy, F. Belleflamme, G. Tabacchi, A. Glöß, M. Lass, I. Bethune, C. J. Mundy, C. Plessl, M. Watkins, J. VandeVondele, M. Krack, and J. Hutter, *The Journal of Chemical Physics* **152**, 194103 (2020).
- [10] J. VandeVondele, M. Krack, F. Mohamed, M. Parrinello, T. Chassaing, and J. Hutter, *Computer Physics Communications* **167**, 103 (2005).
- [11] J. P. Perdew, K. Burke, and M. Ernzerhof, *Physical Review Letters* **77**, 3865 (1996).
- [12] Y. Zhang and W. Yang, *Physical Review Letters* **80**, 890 (1998).
- [13] C. Adamo and V. Barone, *The Journal of Chemical Physics* **110**, 6158 (1999).
- [14] S. Grimme, J. Antony, S. Ehrlich, and H. Krieg, *J. Chem. Phys.* **132**, 154104 (2010).
- [15] T. E. Markland and M. Ceriotti, *Nature Reviews Chemistry* **2**, 1 (2018).
- [16] C. Schran, K. Brezina, and O. Marsalek, *The Journal of Chemical Physics* **153**, 104105 (2020).
- [17] J. Behler and M. Parrinello, *Physical Review Letters* **98**, 146401 (2007).
- [18] J. Behler, *International Journal of Quantum Chemistry* **115**, 1032 (2015).
- [19] T. Morawietz, A. Singraber, C. Dellago, and J. Behler, *Proceedings of the National Academy of Sciences* **113**, 8368 (2016).
- [20] J. Chen, G. Schusteritsch, C. J. Pickard, C. G. Salzmann, and A. Michaelides, *Physical Review B* **95**, 094121 (2017).
- [21] T. Morawietz, O. Marsalek, S. R. Pattenau, L. M. Streacker, D. Ben-Amotz, and T. E. Markland, *The Journal of Physical Chemistry Letters* **9**, 851 (2018).
- [22] T. Ohto, M. Dodia, J. Xu, S. Imoto, F. Tang, F. Zysk, T. D. Kühne, Y. Shigeta, M. Bonn, X. Wu, and Y. Nagata, *The Journal of Physical Chemistry Letters* **10**, 4914 (2019).
- [23] S. Habershon, T. E. Markland, and D. E. Manolopoulos, *The Journal of Chemical Physics* **131**, 024501 (2009).
- [24] G. Imbalzano, Y. Zhuang, V. Kapil, K. Rossi, E. A. Engel, F. Grasselli, and M. Ceriotti, *The Journal of Chemical Physics* **154**, 074102 (2021).

- [25] R. J. Needs, M. D. Towler, N. D. Drummond, and P. L. Rios, *J. Phys.: Condens. Matter* **22**, 023201 (2010).
- [26] R. J. Needs, M. D. Towler, N. D. Drummond, P. López Ríos, and J. R. Trail, *J. Chem. Phys.* **152**, 154106 (2020).
- [27] J. R. Trail and R. J. Needs, *J. Chem. Phys.* **122**, 014112 (2005).
- [28] J. R. Trail and R. J. Needs, *J. Chem. Phys.* **122**, 174109 (2005).
- [29] L. Mitás, E. L. Shirley, and D. M. Ceperley, *J. Chem. Phys.* **95**, 3467 (1991).
- [30] D. Alfè and M. J. Gillan, *Phys. Rev. B* **70**, 161101 (2004).
- [31] A. Zen, S. Sorella, M. J. Gillan, A. Michaelides, and D. Alfè, *Phys. Rev. B* **93**, 241118(R) (2016).
- [32] D. Frenkel and A. J. C. Ladd, *The Journal of Chemical Physics* **81**, 3188 (1984).
- [33] V. Kapil and E. A. Engel, *arXiv:2102.13598 [cond-mat]* (2021), *arXiv: 2102.13598*.
- [34] M. M. Conde, M. A. Gonzalez, J. L. F. Abascal, and C. Vega, *The Journal of Chemical Physics* **139**, 154505 (2013).
